# Supplementary material for: Energy-Preserving Reduced Operator Inference for Efficient Design and Control
Source: arXiv:2401.02889 source file (2024-02-07)
Supplement: Supplementary file 1 [file appendix.tex]

\section*{Appendix}

% A Note on the energy conservation we talked about in class. For Burger's equation
% \begin{equation}
%     \dot u = Au + H(u\otimes u)
% \end{equation}
% where $u$ defines the speed. Then the energy is 
% \begin{equation}
%     \frac{1}{2}\|u\|^2 = \textrm{const.},
% \end{equation}
% if we take the derivative, we have
% \begin{equation}
%     \begin{aligned}
%         \frac{d}{dt}\left(\frac{1}{2}\|u\|^2\right) &= u^\top \dot u = \langle u,\dot u\rangle \\
%         &= \langle u, Au + H(u\otimes u) \rangle \\
%         &= \langle u, Au \rangle + \langle u, H(u\otimes u) \rangle \\
%         &= 0
%     \end{aligned}
% \end{equation}
% Approximate state with projection onto the subspace spanned by the POD basis
% \begin{equation}
%     u \approx V_r\hat u,
% \end{equation}
% Thus,
% \begin{gather}
%     \hat u^\top V_r^\top A V_r \hat u + \hat u^\top V_r^\top H (V_r \otimes V_r)(\hat u \otimes \hat u) = 0\\
%     \hat u^\top \hat A \hat u + \hat u^\top \hat H (\hat u \otimes \hat u) = 0
% \end{gather}
